# Supplementary material for: Public sentiments on the fourth industrial revolution: An unsolicited public opinion poll from Twitter
Source: arXiv:2411.14230 source file (2025-11-27)
Supplement: Supplementary file 1 [file appendix_figures.tex]

%--------------------------------------------------
% APPENDIX FIGURES FOR 4IR PUBLIC SENTIMENT PAPER
% Include in preamble: \usepackage{pgfplots, tikz}
% \pgfplotsset{compat=1.18}
%--------------------------------------------------

\appendix
\section{Supplementary Figures}

%--------------------------------------------------
% FIGURE A1: Sentiment by Technology (7 panels)
%--------------------------------------------------
\begin{figure}[htbp]
\centering
\begin{tikzpicture}
% Row 1: AI, VR, Blockchain
% AI
\begin{axis}[
    name=ai,
    width=5cm, height=3.8cm,
    title={Artificial Intelligence},
    title style={font=\scriptsize},
    xmin=2009, xmax=2019, ymin=0, ymax=1,
    xtick={2010,2015}, xticklabel style={font=\tiny},
    yticklabel style={font=\tiny},
]
\addplot[green!60!black, mark=*, mark size=0.8pt] coordinates {
    (2010,0.85)(2012,0.70)(2014,0.60)(2016,0.50)(2018,0.42)
};
\addplot[blue!70, mark=square*, mark size=0.8pt] coordinates {
    (2010,0.10)(2012,0.20)(2014,0.28)(2016,0.35)(2018,0.42)
};
\addplot[red!70, mark=triangle*, mark size=0.8pt] coordinates {
    (2010,0.05)(2012,0.10)(2014,0.12)(2016,0.15)(2018,0.16)
};
\end{axis}

% VR
\begin{axis}[
    name=vr,
    at={(ai.south east)}, anchor=south west, xshift=0.3cm,
    width=5cm, height=3.8cm,
    title={Virtual Reality},
    title style={font=\scriptsize},
    xmin=2011, xmax=2019, ymin=0, ymax=1,
    xtick={2012,2016}, xticklabel style={font=\tiny},
    yticklabel style={font=\tiny},
]
\addplot[green!60!black, mark=*, mark size=0.8pt] coordinates {
    (2012,0.88)(2014,0.78)(2016,0.72)(2018,0.65)
};
\addplot[blue!70, mark=square*, mark size=0.8pt] coordinates {
    (2012,0.08)(2014,0.15)(2016,0.20)(2018,0.28)
};
\addplot[red!70, mark=triangle*, mark size=0.8pt] coordinates {
    (2012,0.04)(2014,0.07)(2016,0.08)(2018,0.07)
};
\end{axis}

% Blockchain
\begin{axis}[
    name=blockchain,
    at={(vr.south east)}, anchor=south west, xshift=0.3cm,
    width=5cm, height=3.8cm,
    title={Blockchain},
    title style={font=\scriptsize},
    xmin=2013, xmax=2019, ymin=0, ymax=1,
    xtick={2014,2017}, xticklabel style={font=\tiny},
    yticklabel style={font=\tiny},
]
\addplot[green!60!black, mark=*, mark size=0.8pt] coordinates {
    (2014,0.82)(2015,0.70)(2016,0.58)(2017,0.50)(2018,0.45)
};
\addplot[blue!70, mark=square*, mark size=0.8pt] coordinates {
    (2014,0.12)(2015,0.22)(2016,0.32)(2017,0.38)(2018,0.42)
};
\addplot[red!70, mark=triangle*, mark size=0.8pt] coordinates {
    (2014,0.06)(2015,0.08)(2016,0.10)(2017,0.12)(2018,0.13)
};
\end{axis}

% Row 2: Robot, Cloud, IoT
% Robot
\begin{axis}[
    name=robot,
    at={(ai.south west)}, anchor=north west, yshift=-0.8cm,
    width=5cm, height=3.8cm,
    title={Robot},
    title style={font=\scriptsize},
    xmin=2009, xmax=2019, ymin=0, ymax=1,
    xtick={2010,2015}, xticklabel style={font=\tiny},
    yticklabel style={font=\tiny},
]
\addplot[green!60!black, mark=*, mark size=0.8pt] coordinates {
    (2010,0.80)(2012,0.68)(2014,0.58)(2016,0.48)(2018,0.40)
};
\addplot[blue!70, mark=square*, mark size=0.8pt] coordinates {
    (2010,0.12)(2012,0.22)(2014,0.30)(2016,0.38)(2018,0.45)
};
\addplot[red!70, mark=triangle*, mark size=0.8pt] coordinates {
    (2010,0.08)(2012,0.10)(2014,0.12)(2016,0.14)(2018,0.15)
};
\end{axis}

% Cloud
\begin{axis}[
    name=cloud,
    at={(robot.south east)}, anchor=south west, xshift=0.3cm,
    width=5cm, height=3.8cm,
    title={Cloud Computing},
    title style={font=\scriptsize},
    xmin=2009, xmax=2019, ymin=0, ymax=1,
    xtick={2010,2015}, xticklabel style={font=\tiny},
    yticklabel style={font=\tiny},
]
\addplot[green!60!black, mark=*, mark size=0.8pt] coordinates {
    (2010,0.75)(2012,0.68)(2014,0.62)(2016,0.55)(2018,0.50)
};
\addplot[blue!70, mark=square*, mark size=0.8pt] coordinates {
    (2010,0.18)(2012,0.25)(2014,0.30)(2016,0.38)(2018,0.42)
};
\addplot[red!70, mark=triangle*, mark size=0.8pt] coordinates {
    (2010,0.07)(2012,0.07)(2014,0.08)(2016,0.07)(2018,0.08)
};
\end{axis}

% IoT
\begin{axis}[
    name=iot,
    at={(cloud.south east)}, anchor=south west, xshift=0.3cm,
    width=5cm, height=3.8cm,
    title={IoT},
    title style={font=\scriptsize},
    xmin=2009, xmax=2019, ymin=0, ymax=1,
    xtick={2010,2015}, xticklabel style={font=\tiny},
    yticklabel style={font=\tiny},
]
\addplot[green!60!black, mark=*, mark size=0.8pt] coordinates {
    (2010,0.88)(2012,0.78)(2014,0.65)(2016,0.55)(2018,0.48)
};
\addplot[blue!70, mark=square*, mark size=0.8pt] coordinates {
    (2010,0.08)(2012,0.15)(2014,0.25)(2016,0.35)(2018,0.40)
};
\addplot[red!70, mark=triangle*, mark size=0.8pt] coordinates {
    (2010,0.04)(2012,0.07)(2014,0.10)(2016,0.10)(2018,0.12)
};
\end{axis}

% Row 3: 5G (centered)
\begin{axis}[
    name=fiveg,
    at={(cloud.south west)}, anchor=north west, yshift=-0.8cm,
    width=5cm, height=3.8cm,
    title={5G},
    title style={font=\scriptsize},
    xmin=2013, xmax=2019, ymin=0, ymax=1,
    xtick={2014,2017}, xticklabel style={font=\tiny},
    yticklabel style={font=\tiny},
]
\addplot[green!60!black, mark=*, mark size=0.8pt] coordinates {
    (2014,0.90)(2015,0.75)(2016,0.60)(2017,0.50)(2018,0.42)
};
\addplot[blue!70, mark=square*, mark size=0.8pt] coordinates {
    (2014,0.05)(2015,0.15)(2016,0.28)(2017,0.35)(2018,0.40)
};
\addplot[red!70, mark=triangle*, mark size=0.8pt] coordinates {
    (2014,0.05)(2015,0.10)(2016,0.12)(2017,0.15)(2018,0.18)
};
\end{axis}

\end{tikzpicture}
\caption{Sentiment dynamics by 4IR technology. Green: neutral; Blue: positive; Red: negative. All technologies exhibit declining neutrality, though VR shows more stable patterns.}
\label{fig:sentimentbytech}
\end{figure}

%--------------------------------------------------
% FIGURE A2: Sentiment by Theme (5 panels)
%--------------------------------------------------
\begin{figure}[htbp]
\centering
\begin{tikzpicture}
% Employment
\begin{axis}[
    name=employment,
    width=5cm, height=3.8cm,
    title={Employment},
    title style={font=\scriptsize},
    xmin=2009, xmax=2019, ymin=0, ymax=1,
    xtick={2010,2015}, xticklabel style={font=\tiny},
    yticklabel style={font=\tiny},
]
\addplot[green!60!black, mark=*, mark size=0.8pt] coordinates {
    (2010,0.82)(2012,0.70)(2014,0.58)(2016,0.48)(2018,0.40)
};
\addplot[blue!70, mark=square*, mark size=0.8pt] coordinates {
    (2010,0.10)(2012,0.18)(2014,0.28)(2016,0.35)(2018,0.42)
};
\addplot[red!70, mark=triangle*, mark size=0.8pt] coordinates {
    (2010,0.08)(2012,0.12)(2014,0.14)(2016,0.17)(2018,0.18)
};
\end{axis}

% Environment
\begin{axis}[
    name=environment,
    at={(employment.south east)}, anchor=south west, xshift=0.3cm,
    width=5cm, height=3.8cm,
    title={Environment},
    title style={font=\scriptsize},
    xmin=2009, xmax=2019, ymin=0, ymax=1,
    xtick={2010,2015}, xticklabel style={font=\tiny},
    yticklabel style={font=\tiny},
]
\addplot[green!60!black, mark=*, mark size=0.8pt] coordinates {
    (2010,0.80)(2012,0.68)(2014,0.55)(2016,0.45)(2018,0.38)
};
\addplot[blue!70, mark=square*, mark size=0.8pt] coordinates {
    (2010,0.12)(2012,0.22)(2014,0.32)(2016,0.40)(2018,0.45)
};
\addplot[red!70, mark=triangle*, mark size=0.8pt] coordinates {
    (2010,0.08)(2012,0.10)(2014,0.13)(2016,0.15)(2018,0.17)
};
\end{axis}

% Health
\begin{axis}[
    name=health,
    at={(environment.south east)}, anchor=south west, xshift=0.3cm,
    width=5cm, height=3.8cm,
    title={Health},
    title style={font=\scriptsize},
    xmin=2011, xmax=2019, ymin=0, ymax=1,
    xtick={2012,2016}, xticklabel style={font=\tiny},
    yticklabel style={font=\tiny},
]
\addplot[green!60!black, mark=*, mark size=0.8pt] coordinates {
    (2012,0.85)(2014,0.75)(2016,0.65)(2018,0.55)
};
\addplot[blue!70, mark=square*, mark size=0.8pt] coordinates {
    (2012,0.10)(2014,0.18)(2016,0.28)(2018,0.38)
};
\addplot[red!70, mark=triangle*, mark size=0.8pt] coordinates {
    (2012,0.05)(2014,0.07)(2016,0.07)(2018,0.07)
};
\end{axis}

% Other
\begin{axis}[
    name=other,
    at={(employment.south west)}, anchor=north west, yshift=-0.8cm,
    width=5cm, height=3.8cm,
    title={Other},
    title style={font=\scriptsize},
    xmin=2009, xmax=2019, ymin=0, ymax=1,
    xtick={2010,2015}, xticklabel style={font=\tiny},
    yticklabel style={font=\tiny},
]
\addplot[green!60!black, mark=*, mark size=0.8pt] coordinates {
    (2010,0.85)(2012,0.72)(2014,0.60)(2016,0.52)(2018,0.45)
};
\addplot[blue!70, mark=square*, mark size=0.8pt] coordinates {
    (2010,0.08)(2012,0.18)(2014,0.28)(2016,0.35)(2018,0.40)
};
\addplot[red!70, mark=triangle*, mark size=0.8pt] coordinates {
    (2010,0.07)(2012,0.10)(2014,0.12)(2016,0.13)(2018,0.15)
};
\end{axis}

% Privacy
\begin{axis}[
    name=privacy,
    at={(other.south east)}, anchor=south west, xshift=0.3cm,
    width=5cm, height=3.8cm,
    title={Privacy},
    title style={font=\scriptsize},
    xmin=2013, xmax=2019, ymin=0, ymax=1,
    xtick={2014,2017}, xticklabel style={font=\tiny},
    yticklabel style={font=\tiny},
]
\addplot[green!60!black, mark=*, mark size=0.8pt] coordinates {
    (2014,0.78)(2015,0.65)(2016,0.52)(2017,0.45)(2018,0.38)
};
\addplot[blue!70, mark=square*, mark size=0.8pt] coordinates {
    (2014,0.12)(2015,0.22)(2016,0.32)(2017,0.38)(2018,0.42)
};
\addplot[red!70, mark=triangle*, mark size=0.8pt] coordinates {
    (2014,0.10)(2015,0.13)(2016,0.16)(2017,0.17)(2018,0.20)
};
\end{axis}

\end{tikzpicture}
\caption{Sentiment dynamics by thematic domain. Health discourse maintains lower negative sentiment compared to other domains; privacy shows elevated negative sentiment.}
\label{fig:sentimentbytheme}
\end{figure}

%--------------------------------------------------
% FIGURE A3: Echo Chamber by Theme (Panel comparison)
%--------------------------------------------------
\begin{figure}[htbp]
\centering
\begin{tikzpicture}
\begin{axis}[
    width=0.85\textwidth,
    height=6cm,
    xlabel={Year},
    ylabel={Share in Echo Chamber},
    xmin=2009, xmax=2019,
    ymin=0, ymax=0.7,
    xtick={2010,2012,2014,2016,2018},
    ytick={0,0.2,0.4,0.6},
    legend style={at={(0.02,0.98)}, anchor=north west, font=\scriptsize},
    xlabel style={font=\small},
    ylabel style={font=\small},
    grid=major,
    grid style={gray!30},
]
% Employment
\addplot[color=blue!70, mark=*, mark size=1.5pt, thick] coordinates {
    (2010,0.04)(2012,0.12)(2014,0.52)(2016,0.18)(2018,0.22)
};
% Environment
\addplot[color=green!60!black, mark=square*, mark size=1.5pt, thick] coordinates {
    (2010,0.05)(2012,0.15)(2014,0.58)(2016,0.22)(2018,0.25)
};
% Health
\addplot[color=orange!80, mark=triangle*, mark size=1.5pt, thick] coordinates {
    (2012,0.06)(2014,0.45)(2016,0.15)(2018,0.18)
};
% Privacy
\addplot[color=red!70, mark=diamond*, mark size=1.5pt, thick] coordinates {
    (2014,0.48)(2016,0.25)(2018,0.28)
};
% Other
\addplot[color=gray!60, mark=pentagon*, mark size=1.5pt, thick] coordinates {
    (2010,0.03)(2012,0.10)(2014,0.50)(2016,0.17)(2018,0.20)
};
\legend{Employment, Environment, Health, Privacy, Other}
\end{axis}
\end{tikzpicture}
\caption{Echo chamber participation by thematic domain. All themes exhibit the 2014 spike, with privacy and environment showing highest post-spike levels.}
\label{fig:echotheme}
\end{figure}

%--------------------------------------------------
% FIGURE A4: Corpus Size Over Time
%--------------------------------------------------
\begin{figure}[htbp]
\centering
\begin{tikzpicture}
\begin{axis}[
    ybar,
    width=0.85\textwidth,
    height=6cm,
    xlabel={Year},
    ylabel={Number of Tweets},
    xmin=2005.5, xmax=2019.5,
    ymin=0, ymax=18000,
    xtick={2006,2008,2010,2012,2014,2016,2018},
    xticklabel style={font=\small},
    yticklabel style={font=\small},
    xlabel style={font=\small},
    ylabel style={font=\small},
    bar width=0.5cm,
]
\addplot[fill=blue!50, draw=blue!70] coordinates {
    (2006, 50) (2007, 150) (2008, 400) (2009, 1200) (2010, 2800)
    (2011, 5000) (2012, 7500) (2013, 10000) (2014, 12500) (2015, 14000)
    (2016, 15500) (2017, 16500) (2018, 17000) (2019, 16000)
};
\end{axis}
\end{tikzpicture}
\caption{Temporal distribution of corpus. Volume increases substantially after 2010, reflecting both Twitter platform growth and rising public attention to 4IR technologies.}
\label{fig:corpustime}
\end{figure}

%--------------------------------------------------
% FIGURE A5: News vs User Tweet Comparison
%--------------------------------------------------
\begin{figure}[htbp]
\centering
\begin{tikzpicture}
\begin{axis}[
    ybar,
    width=0.85\textwidth,
    height=6cm,
    xlabel={Country},
    ylabel={Number of Tweets (log scale)},
    symbolic x coords={UK, France, Italy, Spain, Germany, Netherlands},
    xtick=data,
    ymode=log,
    log basis y={10},
    ymin=100, ymax=20000,
    xticklabel style={font=\small},
    yticklabel style={font=\small},
    xlabel style={font=\small},
    ylabel style={font=\small},
    bar width=0.35cm,
    legend style={at={(0.98,0.98)}, anchor=north east, font=\small},
]
\addplot[fill=blue!60, draw=blue!80] coordinates {
    (UK, 11651) (France, 9803) (Italy, 4728) (Spain, 4804) 
    (Germany, 1375) (Netherlands, 1209)
};
\addplot[fill=orange!60, draw=orange!80] coordinates {
    (UK, 5922) (France, 5491) (Italy, 3705) (Spain, 3585) 
    (Germany, 852) (Netherlands, 1087)
};
\legend{User Tweets, News Articles}
\end{axis}
\end{tikzpicture}
\caption{Distribution of user tweets and news articles by country. UK and France dominate the corpus; Germany and Netherlands contribute smaller but analytically valuable samples.}
\label{fig:newsvuser}
\end{figure}
